# Supplementary material for: Measurement of Nuclear Transparency Ratios for Protons and Neutrons
Source: arXiv:1811.01823 ancillary file (2019-07-17)
Supplement: Supplementary file 1 [file Transparency_Supp.pdf]

# Measurement of Nuclear Transparency Ratios for Protons and Neutrons

M. Duer et al. (CLAS Collaboration)

Supplementary Material

## 1 Event selection and kinematical distributions

The main challenge in identifying low-$p_{miss}$ and high-$p_{miss}$ $(e, e'n)$ events is the poor neutron momentum resolution. To overcome this obstacle we optimized the event selection cuts using a sample of "smeared protons". We created this sample by smearing the momentum of the proton in each $(e, e'p)$ event by the corresponding neutron momentum resolution.

For each $(e, e'p)$ measured event we raffled several events with "smeared momenta" from a Gaussian distribution with a mean equal to the un-smeared proton momentum and a width equal to the neutron momentum resolution. The neutron momentum resolution in CLAS electromagnetic calorimeter was determined using the exclusive $d(e, e'p\pi^+\pi^-)n$ and $d(e, e'p\pi^+\pi^-n)$ reactions, and is presented in Fig. 1 (left). As can be seen, the neutron momentum resolution is slightly different for neutrons that interact in the different EC layers. Therefore, we generated the smeared protons in fractions that correspond to the probability of the neutrons depositing energy in the different EC layers. Figure 1 (right) shows the difference between the original (un-smeared) and smeared proton momenta. Since different momenta have different resolutions, the resulting distribution is not a simple Gaussian but a sum of Gaussians. The strategy was to use these smeared-protons to help select $(e, e'n)$ events. Below we present details on the two kinematics identification procedures.

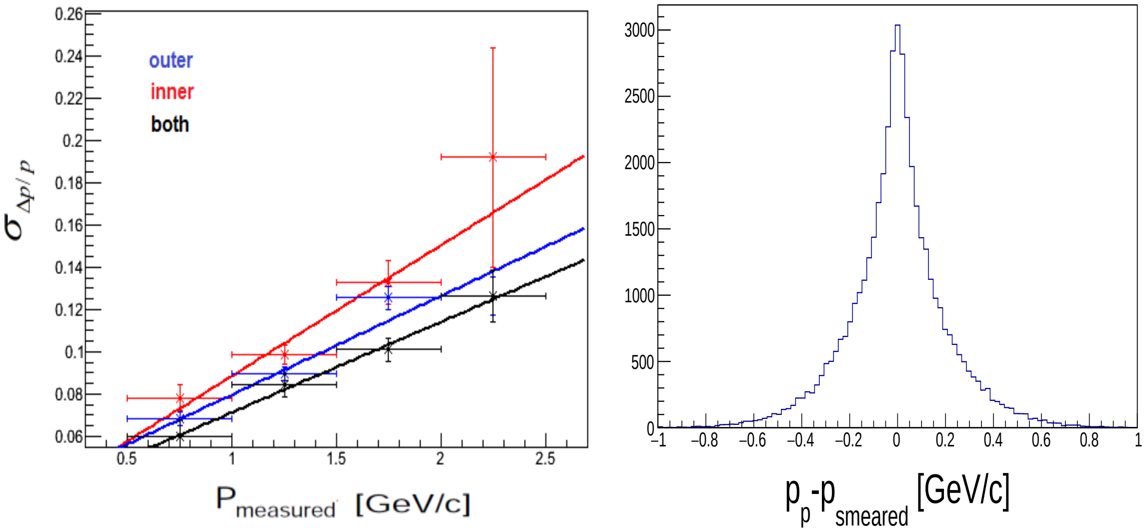


Figure 1: Left: The neutron momentum resolution RMS (the width of the $\Delta p/p$ distribution) as a function of the measured neutron momentum for events detected in the inner, outer and both layers of the EC. Right: The difference between the original (un-smeared) proton momentum ($p_p$) and the smeared proton momentum ($p_{smeared}$).

**Results are shown for C. Similar results are seen for the Al, Fe, and Pb targets.**

## 1.1 Mean-field events

Mean-field (low-$p_{miss}$) events are usually selected based on the missing momentum and missing energy of the event [1-3]. Figure 2 shows the missing energy vs. the missing momentum for $(e, e'n)$ and $(e, e'p)$ events. The latter are shown before and after momentum smearing. A QE peak is clearly observed for the un-smeared $(e, e'p)$ events at $P_{miss} < 0.25$ GeV/c and $E_{miss} < 0.08$ GeV, but is not visible for neutrons or smeared protons due to the poor momentum resolution. Therefore cutting on $E_{miss}$ and $P_{miss}$ will not work.

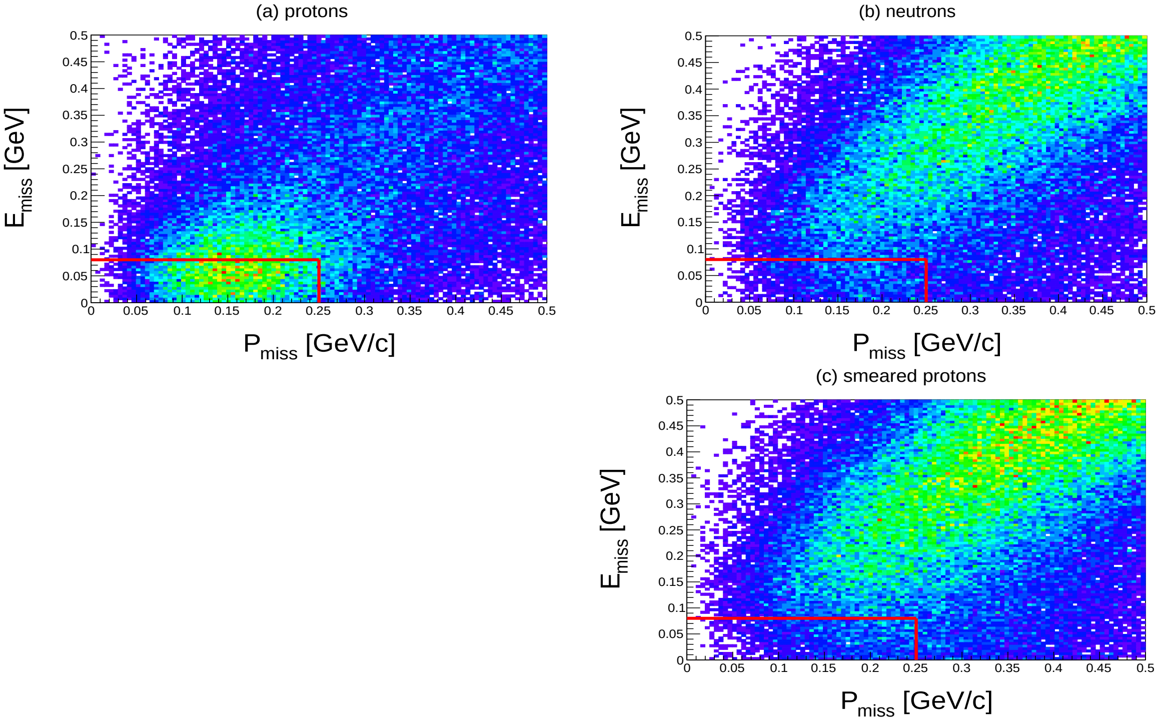


Figure 2: The missing energy vs. the missing momentum for (a) $(e, e'p)$ events, (b) $(e, e'n)$ events and (c) $(e, e'p_{smeared})$ events. The red lines represent the QE (mean-field) region.

To select low missing momentum and missing energy events, we first cut on quantities that are insensitive to the poor neutron momentum resolution, namely the electron kinematic variables and the detected nucleon angle. From the electron variables we can calculate $y$, a scaling variable related to the minimum initial momentum of the knocked-out nucleon in the direction of the momentum transfer:

$$y \equiv \left[ (M_A + \omega)^2 \sqrt{\Lambda^2 - M_{A-1}^2 W^2} - |\vec{q}|\Lambda \right] / W^2 \tag{1}$$

with

$$W = \sqrt{(M_A + \omega)^2 - |\vec{q}|^2} \; , \; \Lambda = \left( M_{A-1}^2 - M_N^2 + W^2 \right) / 2,$$

where $M_A$, $M_{A-1}$ and $M_N$ are, respectively, the masses of the target nucleus, residual nucleus, and nucleon.

Fig. 3 shows the correlations between $y$ and $\omega$, and between $Q^2$ and $\theta_{Nq}$, the angle between the detected nucleon and the momentum transfer vector. The distributions are shown for all events and for low $p_{miss}$ and $E_{miss}$ events (i.e. $p_{miss} < 0.25$ GeV/c and $E_{miss} < 0.08$ GeV) for un-smeared protons. The low missing momentum and energy events populate very narrow parts of the phase-space. We therefore cut on $y$, $\omega$ and $\theta_{Nq}$ un-smeared protons with

low missing momentum and energy:

$$-0.05 < y < 0.25 \tag{2}$$

$$0.95 < \omega < 1.7 \text{ GeV}$$

$$\theta_{pq} < 8^o$$

The $Q^2$ cut shown in Fig. 3 (b) ($1.3 < Q^2 < 3.5$ GeV$^2$/c$^2$) was not implemented.

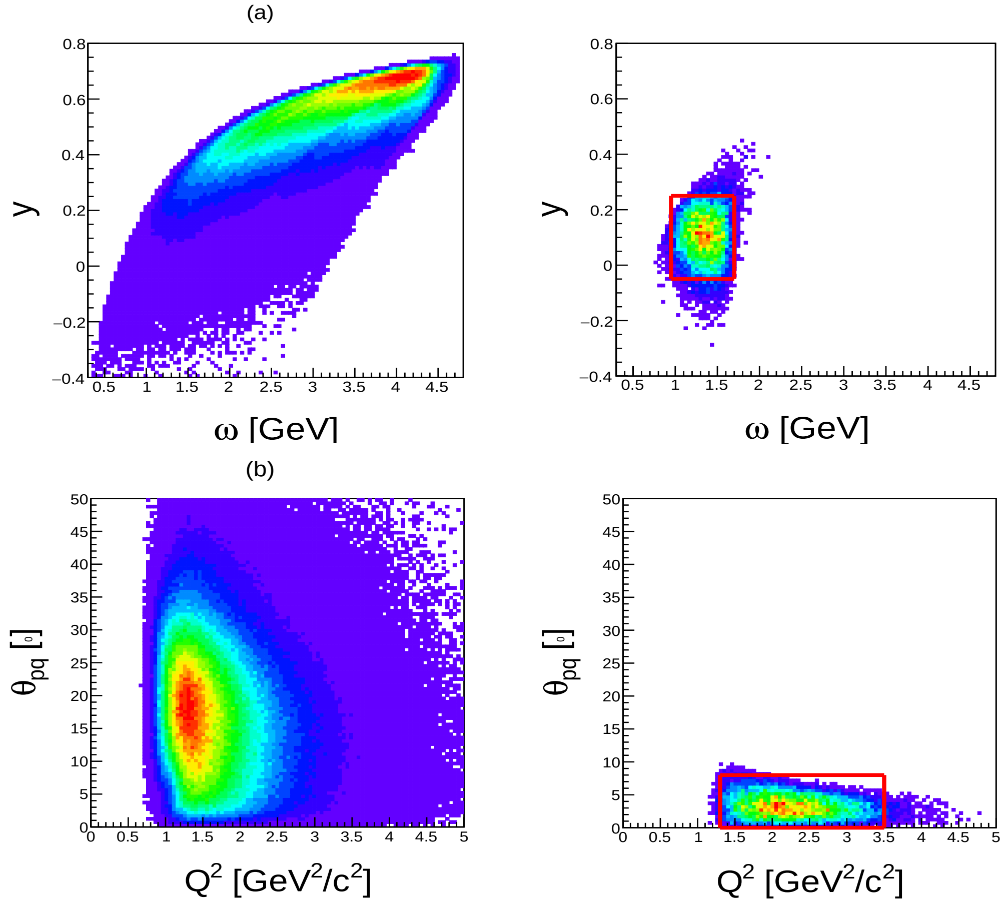


Figure 3: The distribution of un-smeared $(e, e'p)$ events for: (a) the $y$ scaling variable vs. $\omega$ with (right) and without (left) the QE cuts $p_{miss} < 0.25$ GeV/c and $E_{miss} < 0.08$ GeV. (b) same as (a) for $\theta_{pq}$ vs. $Q^2$. The cuts on these variables are marked by the red boxes.

Next, we optimized the cuts on $E_{miss}$ and $p_{miss}$ values using the smeared-proton event sample by varying the cut values and examining:

- False positive probability - The fraction of events that **do pass** the missing momentum and energy cuts using the smeared proton momentum, but **do not pass** the cuts presented above when using the un-smeared momentum. Reducing this fraction maximizes the "purity" of the sample.

- False negative probability - The fraction of events that **do not pass** the missing momentum and energy cuts when using the smeared proton momentum, but **do pass** the equivalent cuts when using their un-smeared momentum. Reducing this fraction maximizes the "efficiency" of the sample.

Figure 4 shows the false positive (left) and false negative (right) probabilities as a function of the missing-momentum cut for different missing-energy cuts applied using the smeared-proton momentum. Based on these, we selected the following cuts for neutrons: $p_{miss} < 300$ MeV/c, $E_{miss} < 190$ MeV. These cuts are in addition to the cuts listed in Eq. 2 above, and lead to false positive and negative probabilities of about 10% and 15% respectively. The sensitivity to the event selection cuts is presented in Table 1.

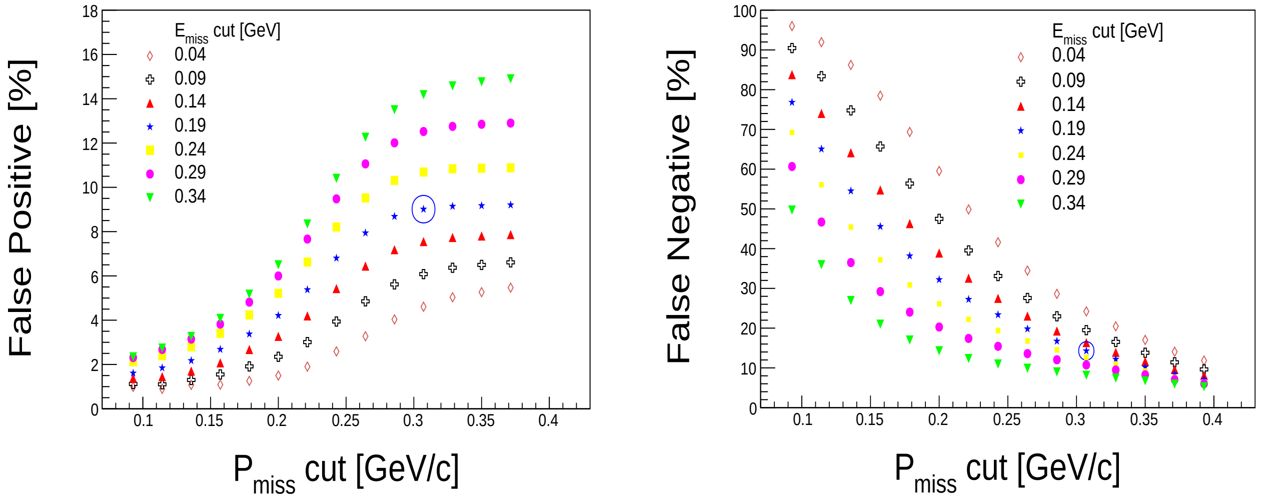


Figure 4: The false positive (left) and negative (right) probabilities for the low missing momentum (QE) events, as a function of the missing momentum cut for different missing energy cuts. The blue circle represents the selected cuts.

| MF Cut | Cut uncertainty [%] | | | | | | |
|---|---|---|---|---|---|---|---|
| | Range | Al/C | | Fe/C | | Pb/C | |
| $-0.05 < y < 0.25$ | $\pm 0.05$ | 1.6 | 0.8 | 1.3 | 1.3 | 1.2 | 1.6 |
| $0.95 < \omega < 1.7$ GeV | $\pm 0.1$ GeV | 1.4 | 1.4 | 0.8 | 1.2 | 2.0 | 1.7 |
| $\theta_{Nq} < 8^\circ$ | $\pm 1^\circ$ | 1.3 | 1.5 | 1.9 | 1.6 | 1.6 | 1.0 |
| $p_{miss} < 0.3$ GeV/c | $\pm 0.025$ GeV/c | 1.2 | 1.2 | 2.0 | 1.3 | 1.8 | 1.5 |
| $E_{miss} < 0.19$ GeV | $\pm 0.02$ GeV | 1.9 | 0.8 | 1.8 | 0.9 | 1.9 | 1.4 |
| | Total: | 3.4 | 2.6 | 3.6 | 2.9 | 3.9 | 3.1 |

Table 1: The $(e, e'N)$event selection cuts for the MF kinematics. Also shown are the uncertainties of each transparency ratio due to variations in the cuts. For each nucleus, the left and the right sensitivity values are for proton and neutron knockout, respectively.

## The distribution of Mean-Field events

We checked that our mean-field event selection cuts functioned as expected and that the distributions of $(e, e,' n)$ and $(e, e'p_{smeared})$ events are the same. Electron scattering from mean-field (low initial momentum) nucleons is kinematically similar to scattering from nucleons at rest. Energy and momentum conservation is given by:

$$(E_{beam}, (0, 0, E_{beam})) + \left(M_N, \vec{0}\right) = \left(E', \vec{P}_{e'}\right) + \left(E_N, \vec{P}_N\right) \quad (3)$$

where $E_{beam}$ is the incoming beam energy, $M_N$ is the nucleon (proton/neutron) mass, $E'$ and $\vec{P}_{e'}$ are the scattered electron energy and momentum respectively, and $E_N$ and $\vec{P_N}$ are the measured nucleon energy and momentum,

respectively. From this equation one can derive the following correlations between the scattered electron ($E'$) and measured nucleon ($N = p/n$) quantities:

$$|\phi_N - \phi_{e'}| = 180^\circ \tag{4}$$

$$\theta_N = cos^{-1}\left(\frac{E - |\vec{p}_{e'}| \cdot cos\theta_{e'}}{|\vec{p}_N|}\right)$$

$$\theta_{e'} = cos^{-1}\left(\frac{E - |\vec{p}_N| \cdot cos\theta_N}{|\vec{p}_{e'}|}\right)$$

$$|\vec{p}_N| = \sqrt{(E + M_N - |\vec{p}_{e'}|)^2 - M_N^2}$$

$$|\vec{p}_{e'}| = \sqrt{(E + M_N - |\vec{p}_N|)^2 - M_N^2}$$

Figure 5 shows the correlation between the momentum of the scattered electron and the knockout nucleon for the selected $(e, e'N)$ events. The red solid line shows the elastic scattering correlation (Eq. 4). As can be seen, the observed QE correlation is as expected from the elastic process. Note that the data is limited by the cuts so this figure is not an evidence for the QE nature of the cuts, rather a check that the cuts were set correctly. Figure 6 shows that the absolute difference between the out of plane scattering angle of the nucleon and the electron is centered around 180°, as expected from Eq. 4. Figure 7 shows the difference between the measured and expected electron (left) and nucleon (right) in-plane scattering angles. The expected scattering angle was calculated assuming Eq. 4. The distributions are overall centered close to zero, however, with a large width due to the momentum resolution.

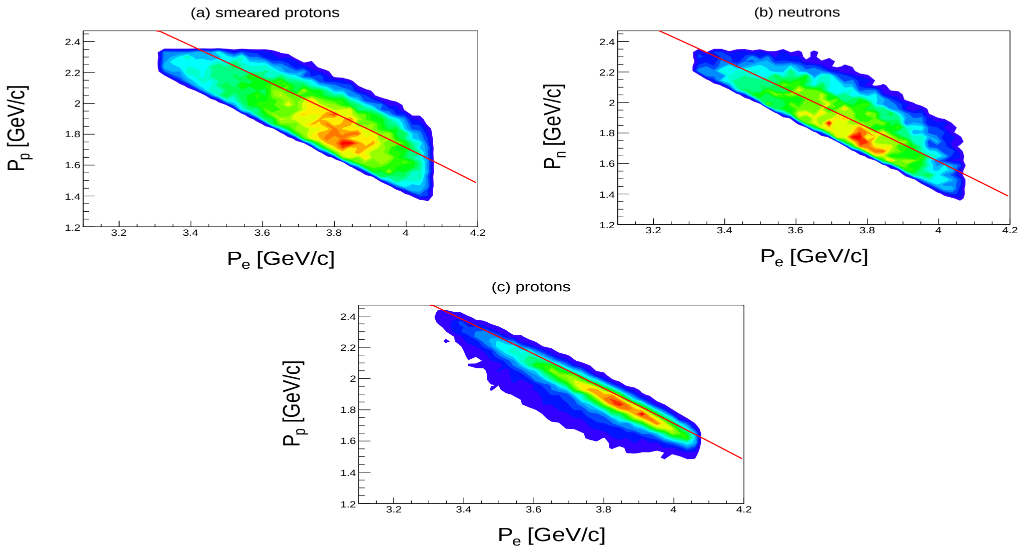


Figure 5: Nucleon vs. electron momentum after applying the MF QE cuts for: (a) $(e, e'p_{smeared})$, (b) $(e, e'n)$, and (c) $(e, e'p)$. The solid red line is the predicted correlation assuming elastic scattering off a stationary free nucleon (Eq. 4).

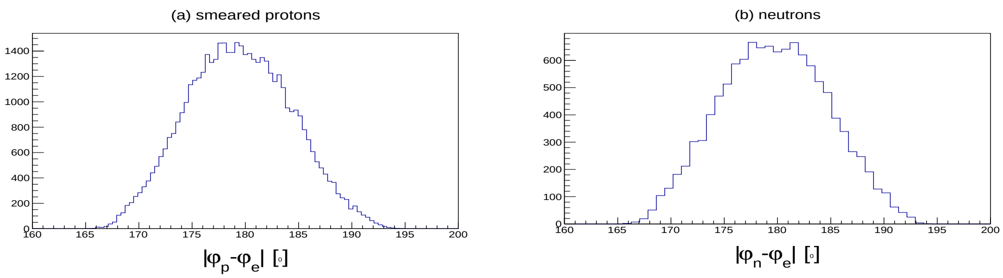


Figure 6: The difference in the out-of-plane scattering angle of the nucleon and the electron after applying the MF QE cuts for: (a) $(e, e'p_{smeared})$ and (b) $(e, e'n)$.

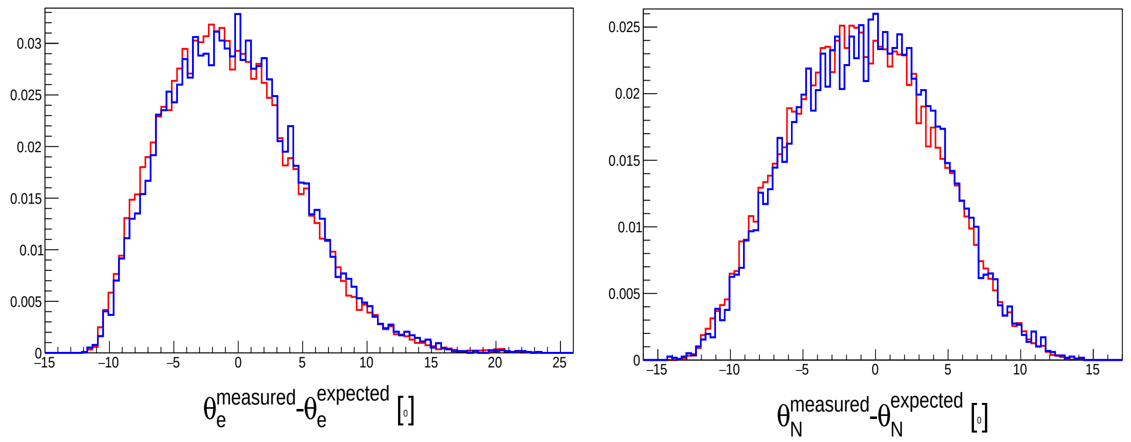


Figure 7: The difference between the measured and expected electron (left) and nucleon (right) scattering angles for smeared protons (red) and neutrons (blue). The expected scattering angles were calculated assuming Eq. 4. The distributions are normalized to unity such that only their shape is compared.

Moreover, in MF QE kinematics, due to large momentum transfer in the reaction, we expect that the final momentum of the knockout nucleon will roughly be equal to the momentum transfer. This can be demonstrated by looking at $\theta_{Nq}$ vs. $\vec{p}_N/\vec{q}$ ratio (Fig. 8). For this purpose only, we did not apply the angular cut ($\theta_{Nq} < 8°$) which is noted by the red lines in Fig. 8. As can be seen, the relative angle is low and the momentum ratio is centered at $\sim 1$.

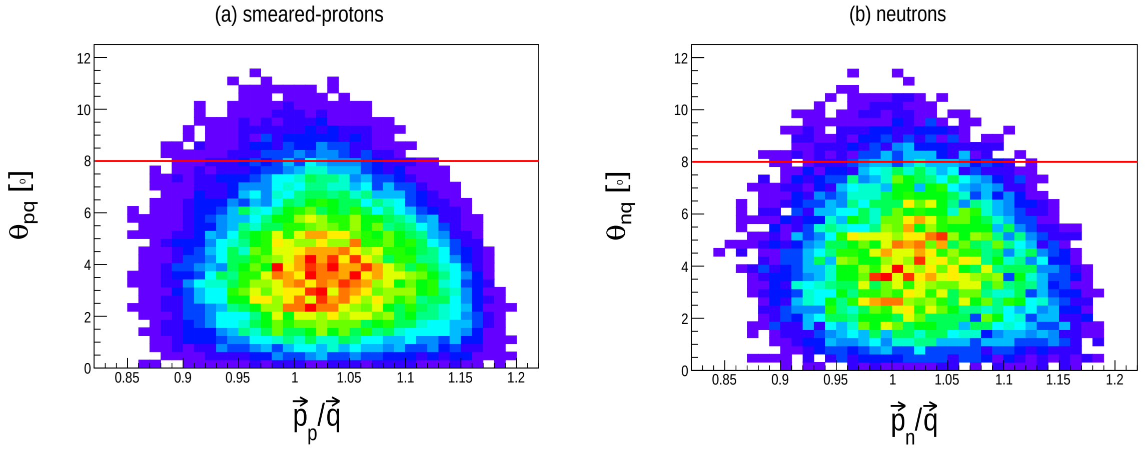


Figure 8: $\theta_{Nq}$ vs. $\vec{p}_N/\vec{q}$ for the selected $(e, e'p_{smeared})$ (a) and $(e, e'n)$ (b) events. Events shown passed all the cuts described above beside the angular cut ($\theta_{Nq} < 8°$) which is noted by the red lines.

Figures 9 and 10 show the kinematical distributions of the resulting $(e, e'n)$ and $(e, e'p)$ (smeared protons) events. As can be seen, the distributions of the MF QE neutrons and smeared protons are similar.

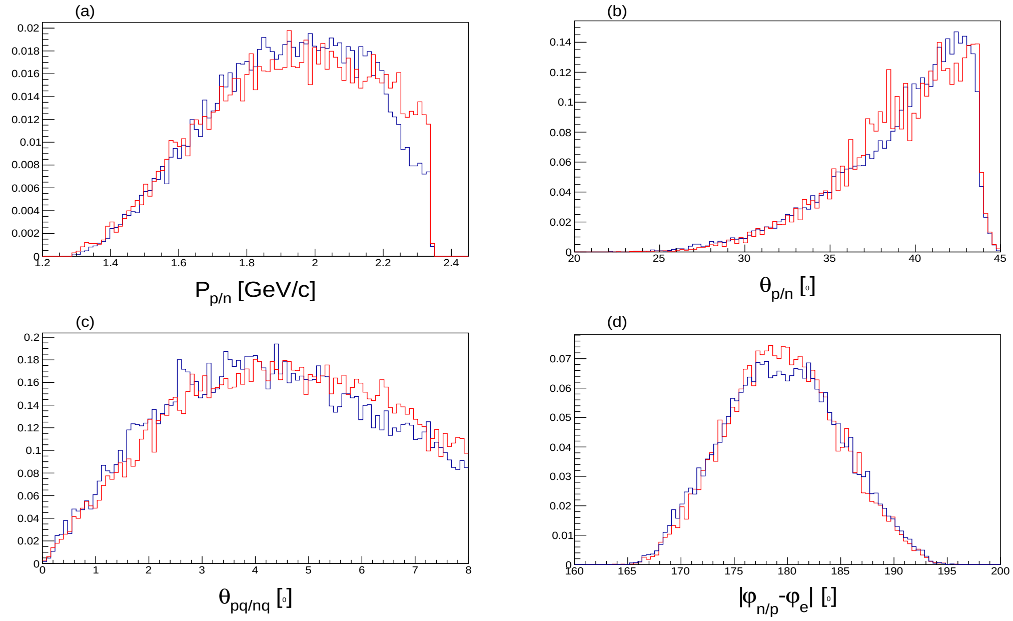


Figure 9: The nucleon kinematic variables for $(e, e'n)$ (blue) and $(e, e'p)$ (smeared protons) (red) after applying the mean-field QE cuts: (a) nucleon momentum, (b) scattering angle, (c) the angle between the nucleon and the momentum transfer vector, and (d) the absolute difference between the out of plane scattering angles of the nucleon and the electron. All distributions are normalized to unity such that only their shape is compared.

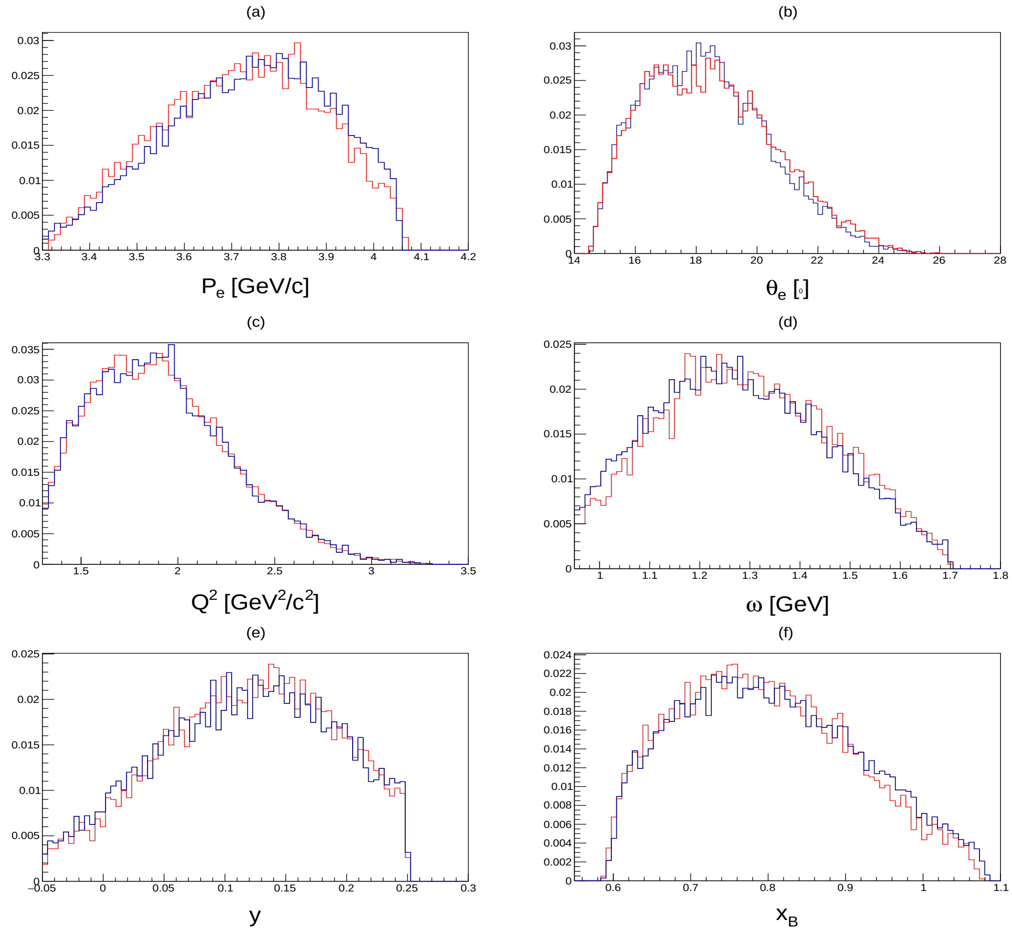


Figure 10: Same as Fig. 9 for the electron kinematic variables: (a) the electron momentum, (b) the electron scattering angle, (c) $Q^2$, (d) $\omega$, (e) $y$, and (f) $x_B$.

## 1.2 SRC events

The identification of SRC (high-$p_{miss}$) $(e, e'p)$ events was previously studied in Ref. [5]. We therefore started by choosing an un-smeared set of $(e, e'p)$ events using the same selection criteria as Ref. [5], and optimized which cuts should be applied to the smeared protons in a similar way as for the mean-field events described above.

The event selection cuts used in Ref. [5], and the modified cuts adapted for this work, are listed in Table 2. The latter include $x_B > 1.1$ (reduced from the 1.2 value used in Ref. [5] to increase statistics), leading nucleon selection ($\theta_{Nq} < 25^\circ$ and $0.62 < |\vec{P}_N|/|\vec{q}| < 1.1$, see Fig. 11) and the two main cuts on the missing momentum and missing mass described below.

| This analysis | Proton analysis [5] |
|---|---|
| $x_B > 1.1$ | $x_B > 1.2$ |
| $0.62 < \|\vec{P}_N\|/\|\vec{q}\| < 1.1$ | $0.62 < \|\vec{P}_N\|/\|\vec{q}\| < 0.96$ |
| $\theta_{N,q} < 25^\circ$ | $\theta_{N,q} < 25^\circ$ |
| $M_{miss} < 1175$ MeV/c$^2$ | $M_{miss} < 1100$ MeV/c$^2$ |
| $400 < p_{miss} < 1000$ MeV/c | $300 < p_{miss} < 1000$ MeV/c |

Table 2: The selected cuts for neutrons ($1^{st}$ column), and the cuts from the protons analysis [5] ($2^{nd}$ column).

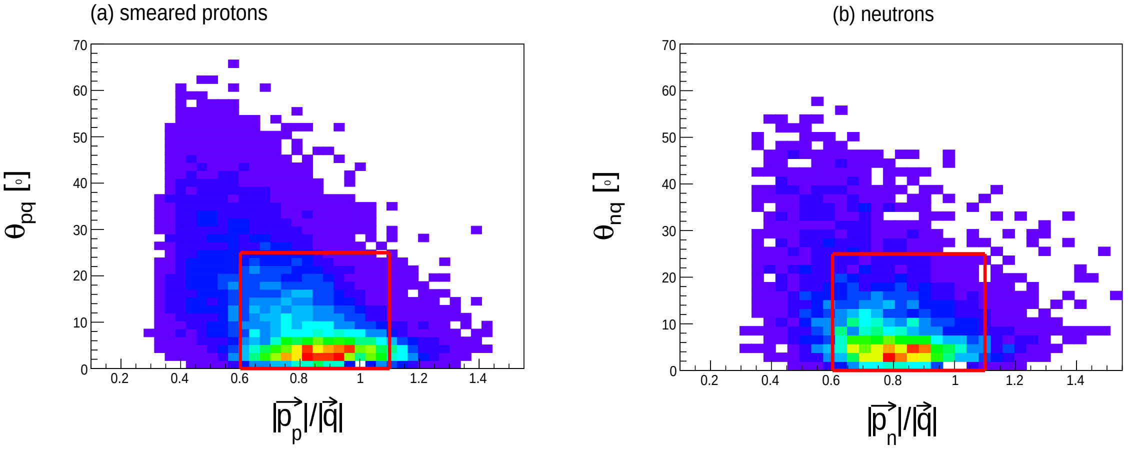


Figure 11: The relative angle between the detected nucleon and the $q$ vector ($\theta_{Nq}$) vs. the ratio between the detected nucleon momentum and the momentum transfer $|\vec{P}_N|/|\vec{q}|$ for events with $x_B > 1.1$. The red box shows the cut applied to select leading nucleons.

If the electron scatters from a pair of nucleons at rest (i.e., $p_{c.m.} = 0$), then the missing mass of the $(e, e'N)$ reaction is: $m^2_{miss} = (q + 2m_N - p_N)^2$. The missing mass, as defined for this reaction should be equal to the nucleon mass. Due to the finite resolution of the detector and the c.m. motion of the pair, the distribution has a finite width and an offset from the real nucleon mass. Figure 12 (a) shows the missing mass distribution from the proton knockout analysis [5]. To avoid contamination from pion-production and delta-excitations Ref. [5] used a cut on a missing mass that is smaller than the center of the distribution + 140 MeV/c$^2$ (i.e. pion mass) i.e., $m_{miss} < 1100$ MeV/c$^2$ (black line in Fig. 12 (a)). Figure 12 (b) shows the missing mass distribution for smeared protons and neutrons.

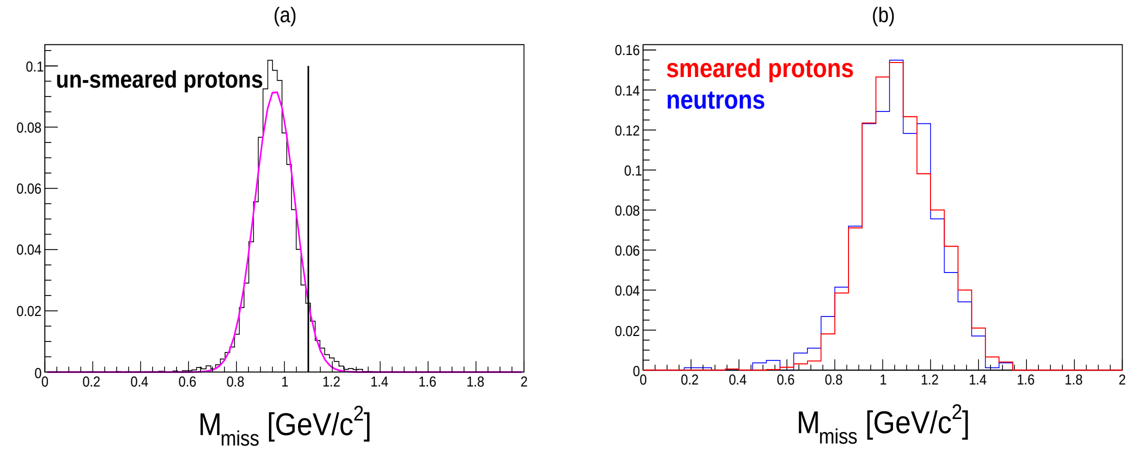


Figure 12: The normalized missing mass distribution for: (a) the proton knockout analysis [5]. The black line indicates the $M_{miss} < 960 + m_\pi = 1100$ GeV/c$^2$ cut applied. The pink line is the Gaussian fit with resulted parameters of $\mu = 0.96 \pm 0.08$ GeV/c$^2$, and $\sigma = 0.08 \pm 0.07$ GeV/c$^2$. (b) smeared protons (red) and neutrons (blue). The events that passed the $x_B$ and the leading nucleon cuts are shown.

In the proton knockout analysis [5] the high missing momentum cut was chosen as: $300 < p_{miss} < 1000$ MeV/c. After applying the $x_B$, and the leading nucleon cuts, we wanted to determine our missing momentum cut. Figure 13 shows the missing momentum distribution for smeared protons and neutrons events. As can be seen, there are almost no events with $p_{miss} > 1000$ GeV/c. We therefore adopt a cut of $p_{miss} < 1000$ MeV/c.

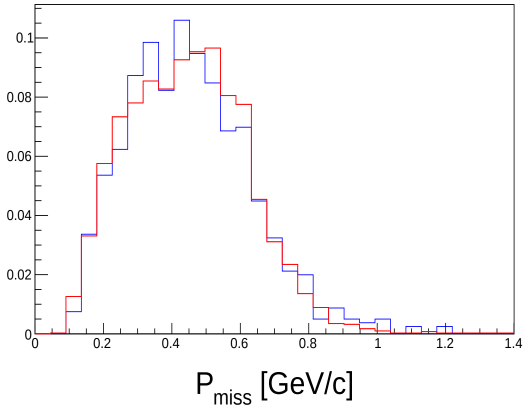


Figure 13: The normalized missing momentum distribution for smeared protons (red) and neutrons (blue). The events shown passed the $x_B$, and the leading nucleon cuts discussed above.

We optimized the main cuts on the lower missing momentum, and missing mass, again, by comparing the smeared protons to the un-smeared protons cuts (see Table 2). Further, we applied different cut combinations and examined the resulting false positive and negative probabilities (see Fig. 14). Based on these rates, we selected the cuts for neutrons ($400 > p_{miss} > 1000$ MeV/c, $m_{miss} < 1175$ MeV/c$^2$), that led to false positive and negative probabilities of about 15% each. The sensitivity to the event selection cuts is presented in Table 3.

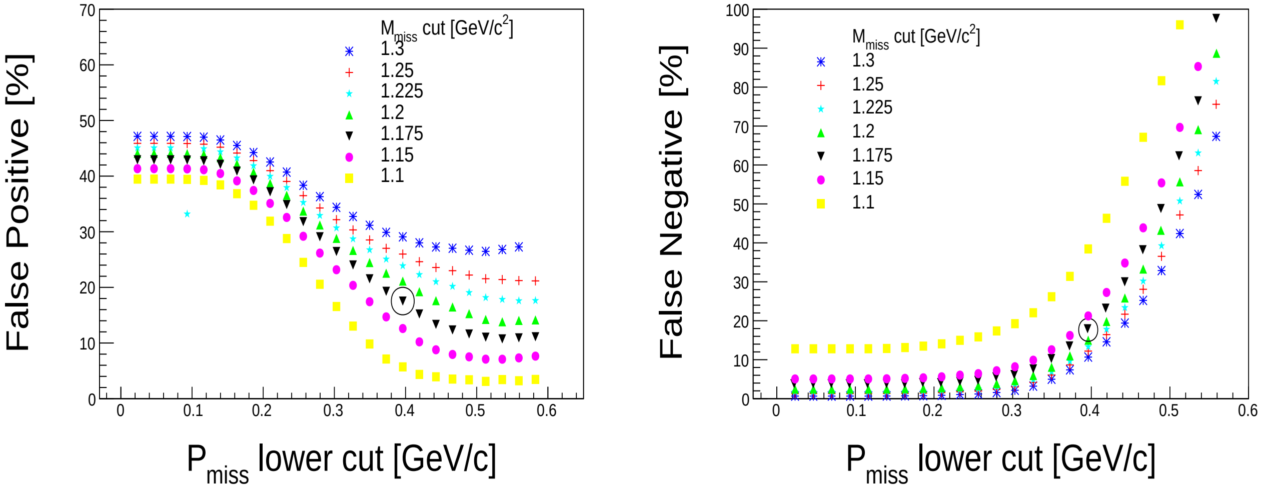


Figure 14: The false positive (left) and negative (right) probabilities, as a function of the smeared protons missing momentum cut for different cuts on the missing mass. The black circles represent the chosen cuts.

| SRC Cut | Cut uncertainty [%] | | | | | | |
|---|---|---|---|---|---|---|---|
| | Range | Al/C | | Fe/C | | Pb/C | |
| $x_B > 1.1$ | $\pm 0.05$ | 0.8 | 1.1 | 1.5 | 2.0 | 2.0 | 1.9 |
| $0.62 < \|\vec{p}_N\|/\|\vec{q}\| < 1.1$<br>$\theta_{Nq} < 25°$ | *$\pm 0.1$ GeV<br>*$\pm 1°$ | 1.4 | 1.4 | 0.8 | 1.2 | 2.0 | 1.7 |
| $m_{miss} < 1.175$ GeV/c$^2$ | $\pm 0.02$ GeV/c$^2$ | 1.9 | 2.4 | 2.1 | 3.0 | 2.2 | 2.0 |
| $0.4 < p_{miss} < 1$ GeV/c | $\pm 0.025$ GeV/c | 2.2 | 2.3 | 1.9 | 1.6 | 2.6 | 2.3 |
| | Total: | 3.6 | 3.8 | 4.1 | 4.7 | 4.6 | 4.4 |

Table 3: Same as Table 1 but for the SRC kinematics. *These cuts were varied together.

### Characterizing the SRC QE selected events

The missing energy of the $(e, e'N)$ reaction is the excitation energy of the residual $(A-1)$ system. To check how well we avoid delta and other resonance production we examine the missing energy distribution. Figure 15 shows the missing energy distributions for the events selected by: (a) the previous proton knockout analysis [5], (b) this analysis, using smeared protons (red) and neutrons (blue), and (c) the un-smeared values for the $(e, e'p)$ events that are shown in (b). As can be seen, the un-smeared proton missing energy distributions do not show an increase at the pion production threshold which would indicate resonance production.

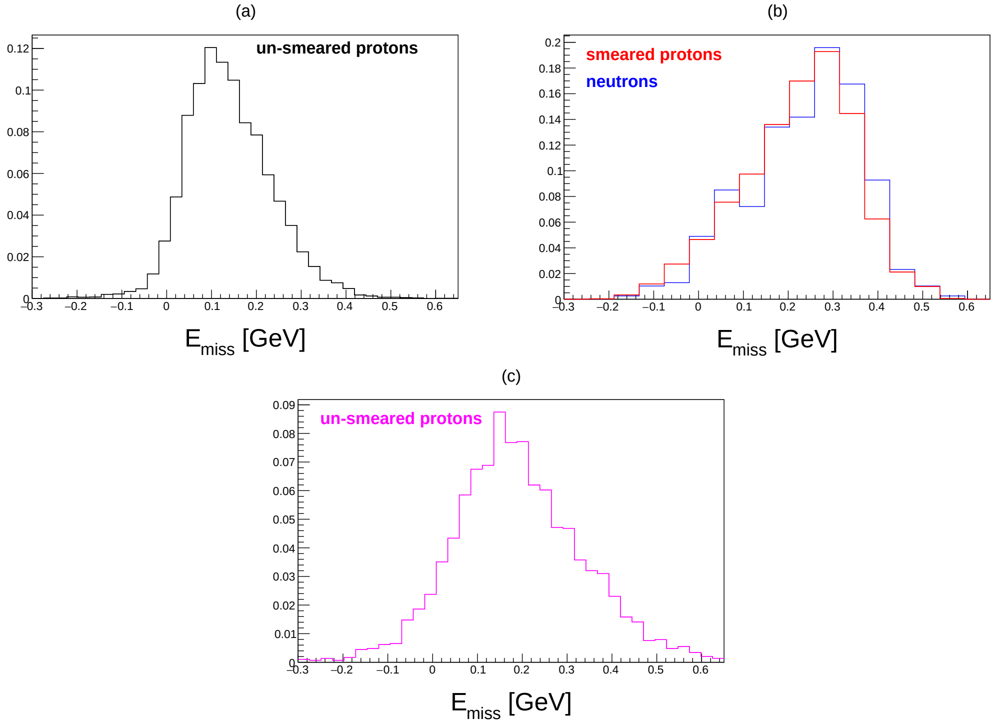


Figure 15: The normalized missing energy distributions for the selected high-momentum QE events of: (a) previous proton knockout analysis [5], (b) this analysis, with smeared protons (red) and neutrons (blue), and (c) the un-smeared values for the $(e, e'p)$ events shown in (b).

Figures 16 and 17 show the kinematical distributions of the resulting $(e, e'n)$ and $(e, e'p)$ (smeared protons) events. As can be seen, the distributions of the SRC QE neutrons and smeared protons are similar.

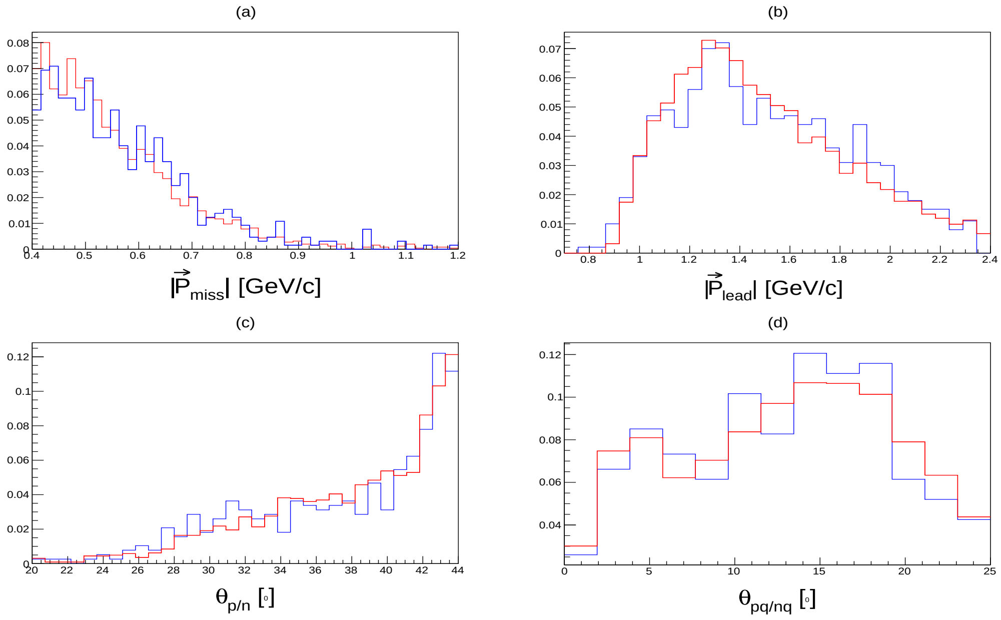


Figure 16: The nucleon kinematic variables for $(e, e'n)$ (blue) and $(e, e'p)$ (smeared protons) (red) after applying the SRC QE cuts: (a) the missing momentum, (b) the leading proton/neutron momentum, (c) the leading proton/neutron scattering angle, and (d) the angle between the struck nucleon and the momentum transfer vector. All distributions are normalized to unity such that only their shapes are to be compared.

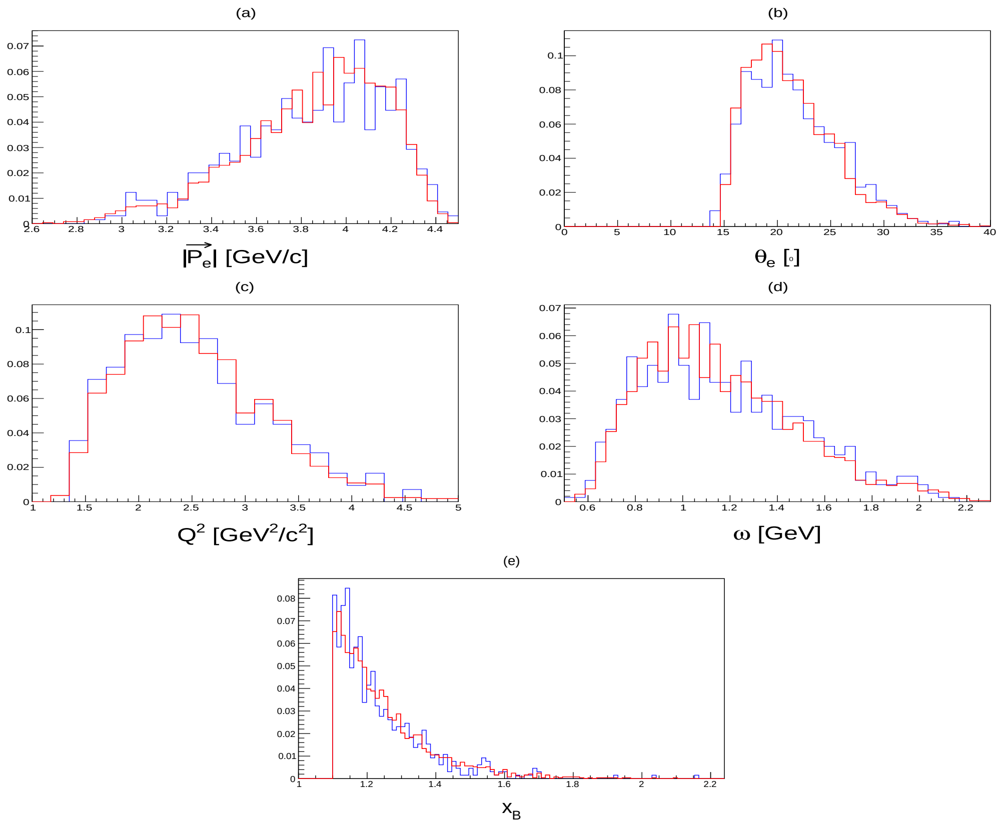


Figure 17: Same as Fig. 16 for the electron kinematic variables: (a) the electron momentum, (b) the electron scattering angle, (c) $Q^2$, (d) $\omega$, and (e) $x_B$.

## 2 Smeared vs. un-smeared proton transparencies

Figure 18 compares the smeared and un-smeared proton transparencies as a function of $A$ for both mean-field (low-$p_{miss}$) and SRC (high-$p_{miss}$) kinematics. The smeared results agree well with the un-smeared proton results indicating that we corrected for bin migration (false positives and false negatives) correctly.

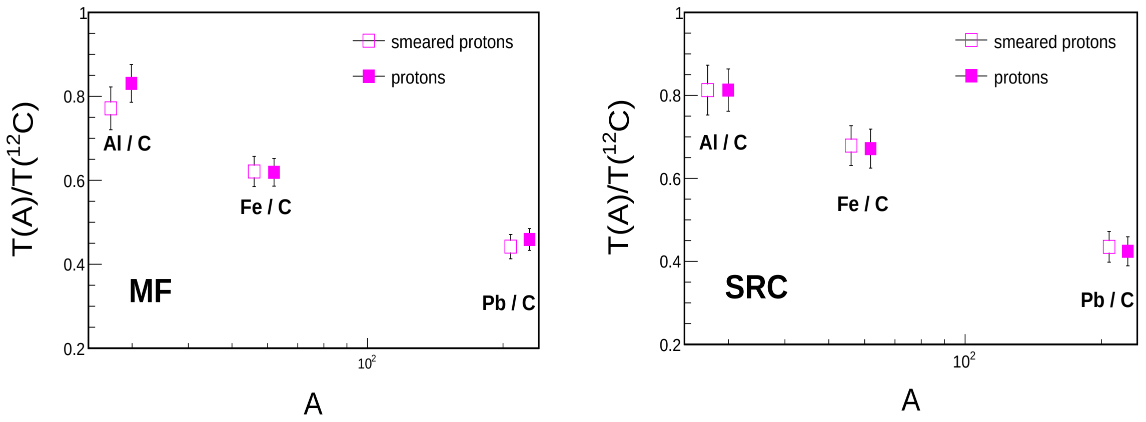


Figure 18: The $A$-dependence of the transparency ratios for smeared and un-smeared protons, for mean-field (left) and high-momentum (right) kinematics.

# References


[1] T.G. Oneill et al., Phys. Lett. B 87, **351** (1995).

[2] D. F. Geesaman et al., Phys. Rev. Lett. **63**, 734 (1989).

[3] G. Garino et al., Phys. Rev. C **45**, 780 (1992).

[4] M. Duer et al., "PROBING 2N-SRC in $^{12}C$, $^{27}Al$, $^{56}Fe$, and $^{208}Pb$ using the $A(e,e'n)$ and $A(e,e'p)$ reactions" , approved CLAS analysis note (2017).http://www-nuclear.tau.ac.il/~eip/neutron3.pdf

[5] O. Hen et al. (CLAS Collaboration), Science **346**, 614 (2014).
